# Supplementary material for: Reducing Variance in Meta-Learning via Laplace Approximation for Regression Tasks
Source: arXiv:2410.01476 source file (2024-10-23)
Supplement: Supplementary file 1 [file ODE_appendix.tex]

\begin{table}[ht]
\centering
\caption{Loss metrics for the Van der Pol oscillator by support size}
\label{tab:vanderpol}
\begin{tabular}{lccc}
\toprule
Model Name & \multicolumn{3}{c}{Support Size} \\
\cmidrule{2-4}
           & 5                & 10               & 20               \\
\midrule
lava\_head         & $2.910 \pm 1.565$ & $1.501 \pm 0.878$ & $1.142 \pm 0.440$ \\
maml\_conditional  & $7.483 \pm 2.438$ & $3.574 \pm 1.186$ & $1.337 \pm 0.595$ \\
vfml               & $9.878 \pm 1.660$ & $6.363 \pm 1.349$ & $4.287 \pm 0.897$ \\
llama              & $11.373 \pm 0.438$ & $6.789 \pm 1.104$ & $4.366 \pm 0.734$ \\
maml\_head         & $19.272 \pm 4.254$ & $12.295 \pm 6.843$ & $7.045 \pm 3.901$ \\
vr                 & $33.686 \pm 7.751$ & $32.265 \pm 6.429$ & $21.513 \pm 4.701$ \\
metamix            & $80.955 \pm 14.401$ & $46.010 \pm 8.290$ & $22.759 \pm 4.856$ \\
\bottomrule
\end{tabular}
\end{table}
